# Supplementary material for: Efficient Speed Planning for Autonomous Driving in Dynamic Environment with Interaction Point Model
Source: arXiv:2209.09013 source file (2022-09-25)
Supplement: Supplementary file 1 [file appendix.tex]

\clearpage
\appendix
\subsection{Qualitative Results\label{appendix:qualitative_results}}

\begin{figure}[htb]
    \vspace{12pt} %<adjust>
    \centering
    \subfloat[Due to the speed limit at $p_o$, the AV slows down from $\text{8.9m/s}$ and has a lower priority than $\text{V}_{228}$ at both $p_1$ and $p_2$.]{
        % \hspace{-0.25in} % offset the previous
        \includegraphics[width=3.0in]{figure/demo2_1.pdf}}

    \centering
    \subfloat[When $\text{V}_{228}$ is going to turn right, the AV decides to occupy $p_1$.]{
        % \hspace{-0.25in} % offset the previous
        \includegraphics[width=3.0in]{figure/demo2_2.pdf}}

    \centering
    \subfloat[Then, the AV follows $\text{V}_{228}$ while maintaining a certain speed.]{
        % \hspace{-0.25in} % offset the previous
        \includegraphics[width=3.0in]{figure/demo2_3.pdf}}

    % \centering
    % \subfloat[The AV follows $\text{V}_{228}$ while maintaining a certain speed.]{
    %     % \hspace{-0.25in} % offset the previous
    %     \includegraphics[width=3.0in]{figure/demo2_4.pdf}}

    \caption{Giving way to other vehicles, where $p_1$ corresponds to a point-overlap, $p_2$ is the first interaction point of a line overlap, and $p_3$ is the location of $V_{213}$. The purple lines are the output speed profiles, and the grey speed profiles are abandoned ones.}
    \label{fig:appendix_qual_result1}
    \vspace{-1em}
\end{figure}

\newpage
\begin{figure}[tb]
    \vspace{43.5pt} %<adjust>
    \centering
    \subfloat[Before passing the intersection, the AV plans to stop before $p_1$ to give way to $V_{232}$.]{
        % \hspace{-0.25in} % offset the previous
        \includegraphics[width=3.0in]{figure/demo1_1.pdf}}
    
    \centering
    \subfloat[Once $\text{V}_{232}$ passes $p_2$, the AV starts to follow it. In the meantime, the AV believes it has a higher priority than $\text{V}_{218}$ at $p_1$.]{
        % \hspace{-0.25in} % offset the previous
        \includegraphics[width=3.0in]{figure/demo1_2.pdf}}

    % \centering
    % \subfloat[The AV successfully overtakes $\text{V}_{218}$]{
    %     % \hspace{-0.25in} % offset the previous
    %     \includegraphics[width=3.0in]{figure/demo1_3.pdf}}

    \centering
    \subfloat[Finally, the AV successfully overtakes $\text{V}_{218}$]{
        % \hspace{-0.25in} % offset the previous
        \includegraphics[width=3.0in]{figure/demo1_4.pdf}}

    \caption{Overtaking other vehicles, where symbols $p_1$ and $p_2$ are in line with those in Fig. \ref{fig:appendix_qual_result1}.}
    \label{fig:appendix_qual_result2}
    \vspace{-1em}
\end{figure}
